# Supplementary material for: On gauge freedom, conservativity and intrinsic dimensionality estimation in diffusion models
Source: arXiv:2402.03845 source file (2024-02-06)
Supplement: Supplementary file 1 [file main_supp.tex]

\documentclass{article}

% if you need to pass options to natbib, use, e.g.:
%     \PassOptionsToPackage{numbers, compress}{natbib}
% before loading neurips_2021

% ready for submission
%\usepackage{neurips_2021}

% to compile a preprint version, e.g., for submission to arXiv, add add the
% [preprint] option:
%     \usepackage[preprint]{neurips_2021}

% to compile a camera-ready version, add the [final] option, e.g.:
%     \usepackage[final]{neurips_2021}

% to avoid loading the natbib package, add option nonatbib:
%\PassOptionsToPackage{sort, numbers}{natbib}	numbers, compress
\usepackage{neurips_2023}
%    [nonatbib]
%    \usepackage[sort, numbers]{natbib}
%%
%	\setcitestyle{square}

\usepackage[utf8]{inputenc} % allow utf-8 input
\usepackage[T1]{fontenc}    % use 8-bit T1 fonts
\usepackage{hyperref}       % hyperlinks
\usepackage{url}            % simple URL typesetting
\usepackage{booktabs}       % professional-quality tables
\usepackage{amsfonts}       % blackboard math symbols
\usepackage{nicefrac}       % compact symbols for 1/2, etc.
\usepackage{microtype}      % microtypography
%\usepackage{xcolor}         % colors

%%%%%%%%%%%%added by me%%%%%%%%%%%%
\usepackage{enumitem,amsmath,amsfonts}

%\newtheorem{question}{Question}
%\usepackage{algorithm,algorithmic}
%\floatname{algorithm}{Algorithm 4: }
%\renewcommand{\algorithmiccomment}[1]{\bgroup\hfill\#~#1\egroup}
%\renewcommand{\algorithmicensure}{\textbf{Initialize:}}

\makeatletter
\makeatother

 %[section]

% for TpX
\usepackage{tikz}
\usepackage{wrapfig}
\usepackage{pstricks}
\usepackage{pgf}
\usepackage{pdfpages, fp}
\usepackage{epic,bez123}
\usepackage{floatflt}
\usepackage{ifpdf}
%%\newcommand*\circled[1]{\tikz[baseline=(char.base)]{
		%	\node[shape=circle,draw,inner sep=2pt] (char) {#1};}}

%\newenvironment{bluebox}
%{\begin{lrbox}{0}\begin{tabular}{@{}l@{}}}
		%		{\end{tabular}\end{lrbox}%
	%	\setlength{\fboxsep}{20pt}% adjust at will
	%	{\centering\fcolorbox{black}{orange}{\usebox{0}}\par}}

%\usepackage{mathtools}
%\let\clipbox\relax
%
%\usepackage{adjustbox}
%\let\clipbox\relax

\usepackage{varwidth}
%\usepackage[most]{tcolorbox}
%
%\newtcbox{bluebox}[1][]{enhanced jigsaw,
	%	sharp corners,
	%	colback=LightSteelBlue,
	%	center,
	%	varwidth upper=0.8\linewidth,
	%	frame hidden,
	%	#1}
%
%\newenvironment{bluebox}{%
	%	\noindent
	%	\adjustbox{innerenv={varwidth}[c]{0.9\linewidth},margin=\fboxsep+.25cm \fboxsep+.2cm,bgcolor=orange,frame,center}\bgroup
	%}{%
	%	\egroup
	%}

%%%%%%%%%%%%%%%%%%%%%%%%%%%%%%%%%%%%
\usepackage{changes}

\title{On the necessity of conservative vector fields in diffusion models - Supplementary}

% The \author macro works with any number of authors. There are two commands
% used to separate the names and addresses of multiple authors: \And and \AND.
%
% Using \And between authors leaves it to LaTeX to determine where to break the
% lines. Using \AND forces a line break at that point. So, if LaTeX puts 3 of 4
% authors names on the first line, and the last on the second line, try using
% \AND instead of \And before the third author name.

\author{%
	Christian Horvat \\
	%	\thanks{Use footnote for providing further information
		%		about author (webpage, alternative address)---\emph{not} for acknowledging
		%		funding agencies.} \\
	Department of Physiology\\
	University of Bern\\
	%	Bern, Switzerland \\
	\texttt{christian.horvat@unibe.ch} \\
	% examples of more authors
	\And
	% Coauthor \\
	Jean-Pascal Pfister \\
	% Affiliation \\
	Department of Physiology \\
	% Address \\
	%	University of Bern\\
	Bern, Switzerland \\
	\texttt{jeanpascal.pfister@unibe.ch} \\
	% \AND
	% Coauthor \\
	% Affiliation \\
	% Address \\
	% \texttt{email} \\
	% \And
	% Coauthor \\
	% Affiliation \\
	% Address \\
	% \texttt{email} \\
	% \And
	% Coauthor \\
	% Affiliation \\
	% Address \\
	% \texttt{email} \\
}

\begin{document}

	%\title{Intrinsic dimensionality estimation using Normalizing Flows}
	
	%\author{\name Christian Horvat \email christian.horvat@unibe.ch \\
		%	\addr Department of Physiology\\
		%	University of Bern\\
		%	Bern, Switzerland
		%	\AND
		%	\name Jean-Pascal Pfister \email jeanpascal.pfister@unibe.ch \\
		%	\addr Department of Physiology\\
		%	University of Bern\\
		%	Bern, Switzerland}
	
	%\editor{ }
	
	\maketitle

	\input{supplementary}
	
	\begin{ack}
		This study has been supported by the Swiss National Science Foundation grant 31003A\_175644.
	\end{ack}
	%%%%REFERENCES
	\bibliographystyle{plain}
	\bibliography{diffusion}
	%\bibliography{references_nips}

	%%%%%%%%%%%%%%%%%%%%%%%%%%%%%%%%%%%%%%%%%%%%%%%%%%%%%%%%%%%%
	
	\newpage

\end{document}
